# Supplementary material for: Learning Is a Kan Extension
Source: arXiv:2502.13810 source file (2025-02-19)
Supplement: Supplementary file 1 [file appendix.tex]

\newpage
\appendix
\onecolumn
\section{appendix}
